# Supplementary material for: DDI-CoCo: A Dataset For Understanding The Effect Of Color Contrast In Machine-Assisted Skin Disease Detection
Source: arXiv:2401.13280 source file (2024-01-24)
Supplement: Supplementary file 1 [file fig_appendix_isic.tex]

\begin{figure}[htbp]
         \centering
         \includegraphics[width=\linewidth]{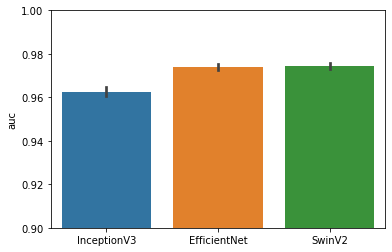}
        
    \caption{\textbf{AUC on ISIC 2019.} We train the three selected models on 80\% of ISIC 2019, and report AUC performance on the rest of the dataset. The reported AUCs are based on results across five different random seeds. EfficientNet and SwinV2 both outperform InceptionNet V3, which again validates our call for adopting more advanced models in this field, as discussed in Sec.~\ref{sec:new_archi}.}
    \label{fig:appendix_isic}
    % \vspace{-5mm}
\end{figure}
